# Supplementary material for: Holography, Supergravity, and the Weak Gravity Conjecture
Source: arXiv:2109.15070 source file (2021-09-30)
Supplement: Supplementary file 1 [file App9.tex]

\noindent Recent work \cite{Cheung:2018cwt, Goon:2019faz} suggests a remarkable universal relationship between the corrections to extremality and corrections to entropy. Here we will present a simple derivation of this relation using standard thermodynamic identities, including a slight generalization of the relation away from extremality. The statement itself is not specific to black holes, and is in fact a relatively universal statement about infinitesimal deformations of thermodynamic systems.  

Consider a thermodynamic system, let $E$ be the total thermal energy, $T$ the temperature, $S$ the entropy and $X$ collectively label a set of extensive thermodynamic variables (for black holes this could be the charge $Q$ and spin $J$). Now consider a small deformation of this system parametrized by a continuous parameter $\epsilon$. The only assumption we will make about this deformation is that it preserves the third law of thermodynamics in the form
\begin{equation}\label{third}
  \lim_{T\rightarrow 0}TS(T,X,\epsilon) = 0,
\end{equation}
for all $\epsilon$ on an open neighbourhood of $\epsilon=0$.

We begin with the first law of thermodynamics in the form
\begin{equation}\label{first}
  1 = T\left(\frac{\partial S}{\partial E}\right)_{X,\epsilon}.
\end{equation}
Making use of the triple product identity
\begin{equation}
  \left(\frac{\partial S}{\partial E}\right)_{X,\epsilon}\left(\frac{\partial E}{\partial \epsilon}\right)_{X,S}\left(\frac{\partial \epsilon}{\partial S}\right)_{X,E} = -1,
\end{equation}
we have 
\begin{equation}
  \left(\frac{\partial E}{\partial \epsilon}\right)_{X,S} = -T \left(\frac{\partial S}{\partial \epsilon}\right)_{X,E}.
\end{equation}
Formally inverting $S(T,X,\epsilon)$ gives $T(S,X,\epsilon)$. We can use this to write 
\begin{equation}
   \left(\frac{\partial E}{\partial \epsilon}\right)_{X,S} =  \left(\frac{\partial E}{\partial \epsilon}\right)_{X,T} +  \left(\frac{\partial E}{\partial T}\right)_{X,\epsilon} \left(\frac{\partial T}{\partial \epsilon}\right)_{X,S}.
\end{equation}
Combining these
\begin{equation}
  \left(\frac{\partial E}{\partial \epsilon}\right)_{X,T} = -T \left(\frac{\partial S}{\partial \epsilon}\right)_{X,E} - \left(\frac{\partial E}{\partial T}\right)_{X,\epsilon} \left(\frac{\partial T}{\partial \epsilon}\right)_{X,S}.
\end{equation}
Next, we use (\ref{first}) again
\begin{align}
  \left(\frac{\partial E}{\partial \epsilon}\right)_{X,T} &= -T \left(\frac{\partial S}{\partial \epsilon}\right)_{X,E} - \left(\frac{\partial E}{\partial T}\right)_{X,\epsilon} \left(\frac{\partial T}{\partial \epsilon}\right)_{X,S} \nonumber\\
                                                          &=-T \left(\frac{\partial S}{\partial \epsilon}\right)_{X,E} - T\left(\frac{\partial S}{\partial E}\right)_{X,\epsilon}\left(\frac{\partial E}{\partial T}\right)_{X,\epsilon} \left(\frac{\partial T}{\partial \epsilon}\right)_{X,S} \nonumber\\
                                                          &=-T \left(\frac{\partial S}{\partial \epsilon}\right)_{X,E} - T\left(\frac{\partial S}{\partial T}\right)_{X,\epsilon} \left(\frac{\partial T}{\partial \epsilon}\right)_{X,S},
\end{align}
one final application of the triple product identity gives the \textit{generalized Goon-Penco relation}
\begin{equation}\label{result}
   \left(\frac{\partial E}{\partial \epsilon}\right)_{X,T} +T \left(\frac{\partial S}{\partial \epsilon}\right)_{X,E} = T \left(\frac{\partial S}{\partial \epsilon}\right)_{X,T}.
\end{equation}
Next we make use of the assumption that the deformation does not violate the third law of thermodynamics. Taylor expanding (\ref{first}) we have
\begin{equation}
  \lim_{T\rightarrow 0} \left[TS(T,X,\epsilon=0) + \epsilon T \left(\frac{\partial S}{\partial \epsilon}\right)_{T,X}\biggr\vert_{\epsilon=0} +\mathcal{O}\left(\epsilon^2\right)\right] = 0.
\end{equation}
By assumption this is true on an open neighbourhood of $\epsilon=0$ and so must be true order-by-order in the expansion, this gives
\begin{equation}
  \lim_{T\rightarrow 0} T\left(\frac{\partial S}{\partial \epsilon}\right)_{T,X}\biggr\vert_{\epsilon=0} = 0 \, .
\end{equation}
Using this together with (\ref{result}) gives the Goon-Penco relation
\begin{equation}
      \boxed{\lim_{T\rightarrow 0}\left[\left(\frac{\partial E}{\partial \epsilon}\right)_{X,T}\biggr\vert_{\epsilon=0} +T \left(\frac{\partial S}{\partial \epsilon}\right)_{X,E}\biggr\vert_{\epsilon=0}\right] = 0.}
\end{equation}
For the specific application to black hole thermodynamics we identify $E$ with the mass $M$ of the black hole, $X$ with the black hole parameters measured at infinity such as charge $Q$ or angular momentum $J$, and $\epsilon$ with a Wilson coefficient of a four-derivative effective operator. 

In section III, we have pointed out that shift in charge at fixed mass is also proportional to the entropy shift and mass shift. This statement can be derived similarly. By the triple product identity, 
\begin{align}
\begin{split}
    \left( \frac{\partial E}{\partial \epsilon} \right)_{X_i, T} = - \left( \frac{\partial X_i}{\partial \epsilon} \right)_{E, T} \left( \frac{\partial E}{\partial X_i} \right)_{\epsilon, T} \, .
\end{split}
\end{align}
This holds for any extensive quantity. Now we choose $X_i = Q$, and we may identify 
\begin{align}
    \left( \frac{\partial E}{\partial X_i} \right)_{\epsilon, T} = \Phi.
\end{align}
So we find 
\begin{align}
\begin{split}
    \left( \frac{\partial E}{\partial \epsilon} \right)_{Q, T} =  -\Phi \left( \frac{\partial Q}{\partial \epsilon} \right)_{E, T}.
\end{split}
\end{align}
For black holes, this means that the shift in charge is related to the shift in mass.  Neither of them is related to the entropy except at extremality. The result of this is that the entropy shift at extremality may be related to the extremality shift at constant charge or at constant mass,
\begin{align}
    \lim_{T\rightarrow 0} \left( \frac{\partial E}{\partial \epsilon} \right)_{Q, T} = - \lim_{T\rightarrow 0}  \Phi \left( \frac{\partial Q}{\partial \epsilon} \right)_{E, T} =  - \lim_{T\rightarrow 0} T \left(\frac{\partial S}{\partial \epsilon}\right)_{Q,E}.
\end{align}

\section{Comment on $\alpha'$-Corrections to Black Holes in Heterotic String Theory }

\noindent Recent work has considered the leading $\alpha'$-corrections to dyonic Reissner-Nordstr{\"o}m black holes embedded in heterotic string theory \cite{Cano:2019oma, Cano:2019ycn}. Though the four-dimensional backgrounds considered in these papers are asymptotically flat, we would like to briefly comment on them in connection with the universal entropy-extremality relationship.

From the dimensionally reduced, effective four-dimensional solutions the authors calculated explicit expressions for the Wald entropy, 
\begin{equation}
   S =  \pi  \left[\left(\mu +M\right)^2+\epsilon  \alpha ' \frac{\left(18 M \mu+21
   \mu^2 +M^2\right)}{40 \mu
   \left(\mu+M\right)}
   \right],
\end{equation}
and Hawking temperature,
\begin{equation} \label{alphaT}
    T =\frac{\mu}{2 \pi
    \left(\mu + M \right)^2}+\epsilon  \alpha '\frac{ \left(M + 3 \mu \right)
   \left( M-\mu \right)^2}{160 \pi  \mu
   \left(\mu +M \right)^5},
\end{equation}
where we have defined $\mu = \sqrt{M^2-\frac{P^2}{2}}$. Here $P$ denotes the charge of the black hole, and we have adopted the same small expansion parameter $\epsilon$ as earlier. From these results it is straightforward to verify the following relation 
\begin{equation}
    T^{-1} = \left(\frac{\partial S}{ \partial M}\right)_P,
\end{equation}
up to errors of $\mathcal{O}(\epsilon^2)$. Consequently, the parameter $M$ corresponds to the thermal mass of the black hole. With these explicit expressions we can verify the entropy-extremality relation derived in \cite{Goon:2019faz}. The differential change in the mass at fixed temperature is given by a simple application of the triple product identity,
\begin{equation} \label{alphaDM}
   \left(\frac{\partial M}{\partial \epsilon}\right)_{T,P} = -\frac{\left(\frac{\partial T}{\partial \epsilon}\right)_{M,P}}{\left(\frac{\partial T}{\partial M}\right)_{\epsilon,P}}\biggr\vert_{\epsilon=0}.
\end{equation}
The differential change in the \textit{extremal} mass is given by taking $T\rightarrow 0^+$. This limit must be taken indirectly since the function (\ref{alphaT}) is too complicated to be inverted directly. The zero temperature limit is then the same as taking $M\rightarrow M_{\text{ext}}$. Since (\ref{alphaDM}) is already a relation between two quantities at $\mathcal{O}(\alpha')$, we only require  $M\rightarrow (M_{\text{ext}})_0$, which is the leading-order extremality relationship
\begin{equation}
    (M_{\text{ext}})_0 = \frac{|P|}{\sqrt{2}}.
\end{equation}
The correction to the extremal mass is then found to be
\begin{equation}
    \left(\frac{\partial M}{\partial \epsilon}\right)_{T = 0,P} = -\frac{\alpha'}{40\sqrt{2}|P|},
    \label{cano_mass}
\end{equation}
in agreement with \cite{Cano:2019ycn}.
To verify the entropy-extremality relation we also need the shift to the entropy at fixed charge and mass. Since the Wald entropy given above is already parametrized in terms of the thermal mass and charge, this is trivial to calculate,
\begin{equation}
    \left(\frac{\partial S}{\partial \epsilon}\right)_{M,P} =   \alpha '\pi \frac{\left(M^2 + 18 M \mu +21
   \mu^2 \right)}{40 \mu
   \left(\mu +M\right)}.
\end{equation}
According to \cite{Goon:2019faz}, we should take the zero temperature limit of this expression multiplied by the uncorrected temperature. This is equivalent to taking $M\rightarrow (M_{\text{ext}})_0$. 
Indeed, taking this limit we find
\begin{equation}
\label{T0DeltaS}
    \lim_{T\rightarrow 0} T_0 \left(\frac{\partial S}{\partial \epsilon}\right)_{M,P} = \lim_{M\rightarrow (M_{\text{ext}})_0} \;\lim_{\epsilon \rightarrow 0} \;T(M,P,\epsilon) \left(\frac{\partial S}{\partial \epsilon}\right)_{M,P} = \frac{\alpha'}{40\sqrt{2}|P|}\, ,
\end{equation}
which agrees precisely with the shift to the mass in (\ref{cano_mass}), verifying the entropy-extremality relationship.  
While (\ref{T0DeltaS}) was also reproduced in \cite{Cano:2019ycn}, the authors suggest that it may be more convenient to work in a near-extremal regime, in which the result of \cite{Goon:2019faz}
would be modified.
In particular, in the ``very near-extremal" regime  discussed in \cite{Cano:2019ycn}, in which one extracts the leading order terms in the near extremal temperature and near extremal entropy (both contributions of order $\sqrt{\epsilon}$), one
finds 
$\frac{\alpha'}{80\sqrt{2}|P|}$,
which differs from
(\ref{T0DeltaS}) precisely by a factor of $1/2$.

Such issues are related to the claim 
of \cite{Cano:2019ycn} that the positivity of the 
entropy shift 
doesn't necessarily imply a positive correction 
to the charge to mass ratio at extremality.
Here we would like to further clarify the 
validity of the results of \cite{Goon:2019faz}, 
and stress that the order of limits 
was \emph{crucial} in order to obtain (\ref{T0DeltaS}).
Indeed, if the limits were taken in 
the other order, we would find
\begin{equation}
    \lim_{\epsilon \rightarrow 0}\;\lim_{M\rightarrow M_{\text{ext}}}  \;T(M,P,\epsilon) \left(\frac{\partial S}{\partial \epsilon}\right)_{M,P} = \frac{\alpha'}{60\sqrt{2}|P|},
\end{equation}
which does not agree with the correction to the extremal mass. The near-extremal computation that yields the $1/2$ factor mentioned above is yet another way to compute $T \Delta S$, which not surprisingly leads to a different value. The final result is indeed extremely sensitive to the
way in which one approaches extremality. 
Nonetheless, the results of \cite{Goon:2019faz} are valid in general,  provided the extremality limit is taken in a  precise way, as described by (\ref{T0DeltaS}).
