# Supplementary material for: Holography, Supergravity, and the Weak Gravity Conjecture
Source: arXiv:2109.15070 source file (2021-09-30)
Supplement: Supplementary file 2 [file App3.tex]

The bosonic matter content of type IIB supergravity consist of the NSNS fields $g_{\mu\nu}$, $B_{\mu\nu}$ and $\phi$ and the RR fields $\chi\equiv C_0$, $C_2$ and $C_4$.  The field strengths obtained from these potentials are defined by:
\begin{align}
    F_1 &= d \chi, \qquad  \qquad H_3 = d B_2, \qquad  \qquad F_3 = dC_2 \, - \chi H_3,\nn \\
    F_5 &= d C_4 - \frac{1}{2} \, ( \, C_2 \wedge \, H_3 \, - B_2 \, \wedge \, d C_2 \, ),
\end{align}
where $F_5$ is self-dual, $F_5=*F_5$.  The Bianchi identities then follow:
\begin{align}
    d F_1 &= 0, \qquad \qquad d F_3 - H_3 \wedge F_1 = 0,\nn \\
    d H_3 &= 0, \qquad \qquad d F_5 - H_3 \wedge F_3 = 0
\end{align}

Type IIB supergravity does not admit a covariant action because of the self-duality of $F_5$.  However, we can write down the equations of motion.  The form field equations are
\begin{align}
    d( e^{2 \phi} * F_1) &=- e^{\phi} H_3 \wedge * F_3,\nn\\
    d*d\phi &= e^{2 \phi} F_1 \wedge * F_1 - \ft12 e^{- \phi} H_3 \wedge * H_3+\ft12 e^{\phi} F_3 \wedge * F_3,\nn \\
    d( e^{- \phi} * H_3) &=e^{\phi} F_1 \wedge * F_3 +F_3 \wedge F_5,\nn\\
    d( e^{\phi} * F_3) &=-H_3 \wedge F_5,
\end{align}
and the Einstein equation in Ricci form is
%%%%
\begin{align}
    R_{\mu\nu}&=\fft12\partial_\mu\phi\partial_\nu\phi+\fft12e^{2\phi}\partial_\mu\chi\partial_\nu\chi+\fft14e^{-\phi}\left(H_{\mu\rho\sigma}H_\nu{}^{\rho\sigma}-\fft1{12}g_{\mu\nu}H_{\lambda\rho\sigma}H^{\lambda\rho\sigma}\right)\nn\\
    &\qquad+\fft14e^\phi\left(F_{\mu\rho\sigma}F_\nu{}^{\rho\sigma}-\fft1{12}g_{\mu\nu}F_{\lambda\rho\sigma}F^{\lambda\rho\sigma}\right)+\fft1{4\cdot4!}F_{\mu\lambda\rho\sigma\tau}F_\nu{}^{\lambda\rho\sigma\tau}.
\end{align}
%%%%

The above equations can reexpressed in terms of the complex fields
\begin{equation}
    \tau=\chi+ie^{-\phi},\qquad G_3=F_3-ie^{-\phi}H_3.
\end{equation}
In particular, we have
\begin{align}
    \fft{d*d\tau}{\tau_2}+i\fft{d\tau\wedge*d\tau}{\tau_2^2}&=-\fft{i}{2\tau_2}G_3\wedge*G_3,\nn\\
    d*G_3&=-i\fft{d\tau}{\tau_2}\wedge*\Re G_3+iF_5\wedge G_3,\nn\\
    dF_5&=\fft{i}{2\tau_2}G_3\wedge \overline{G}_3,
\end{align}
along with
\begin{equation}
    R_{\mu\nu}=\fft1{2\tau_2^2}\partial_{(\mu}\tau\partial_{\nu)}\bar\tau+\fft14\left(G_{(\mu}{}^{\rho\sigma}\overline{G}_{\nu)\rho\sigma}-\fft1{12}g_{\mu\nu}G_{\lambda\rho\sigma}\overline{G}^{\lambda\rho\sigma}\right)+\fft1{4\cdot4!}F_{\mu\lambda\rho\sigma\tau}F_\nu{}^{\lambda\rho\sigma\tau}.
\end{equation}
Here the overlines indicate complex conjugation.
